# Supplementary material for: A Vector Quantized Approach for Text to Speech Synthesis on Real-World Spontaneous Speech
Source: arXiv:2302.04215 source file (2023-02-08)
Supplement: Supplementary file 1 [file appendix-transformertts.tex]

\begin{figure*}[!t]
    \centering
    \includegraphics[width=\textwidth]{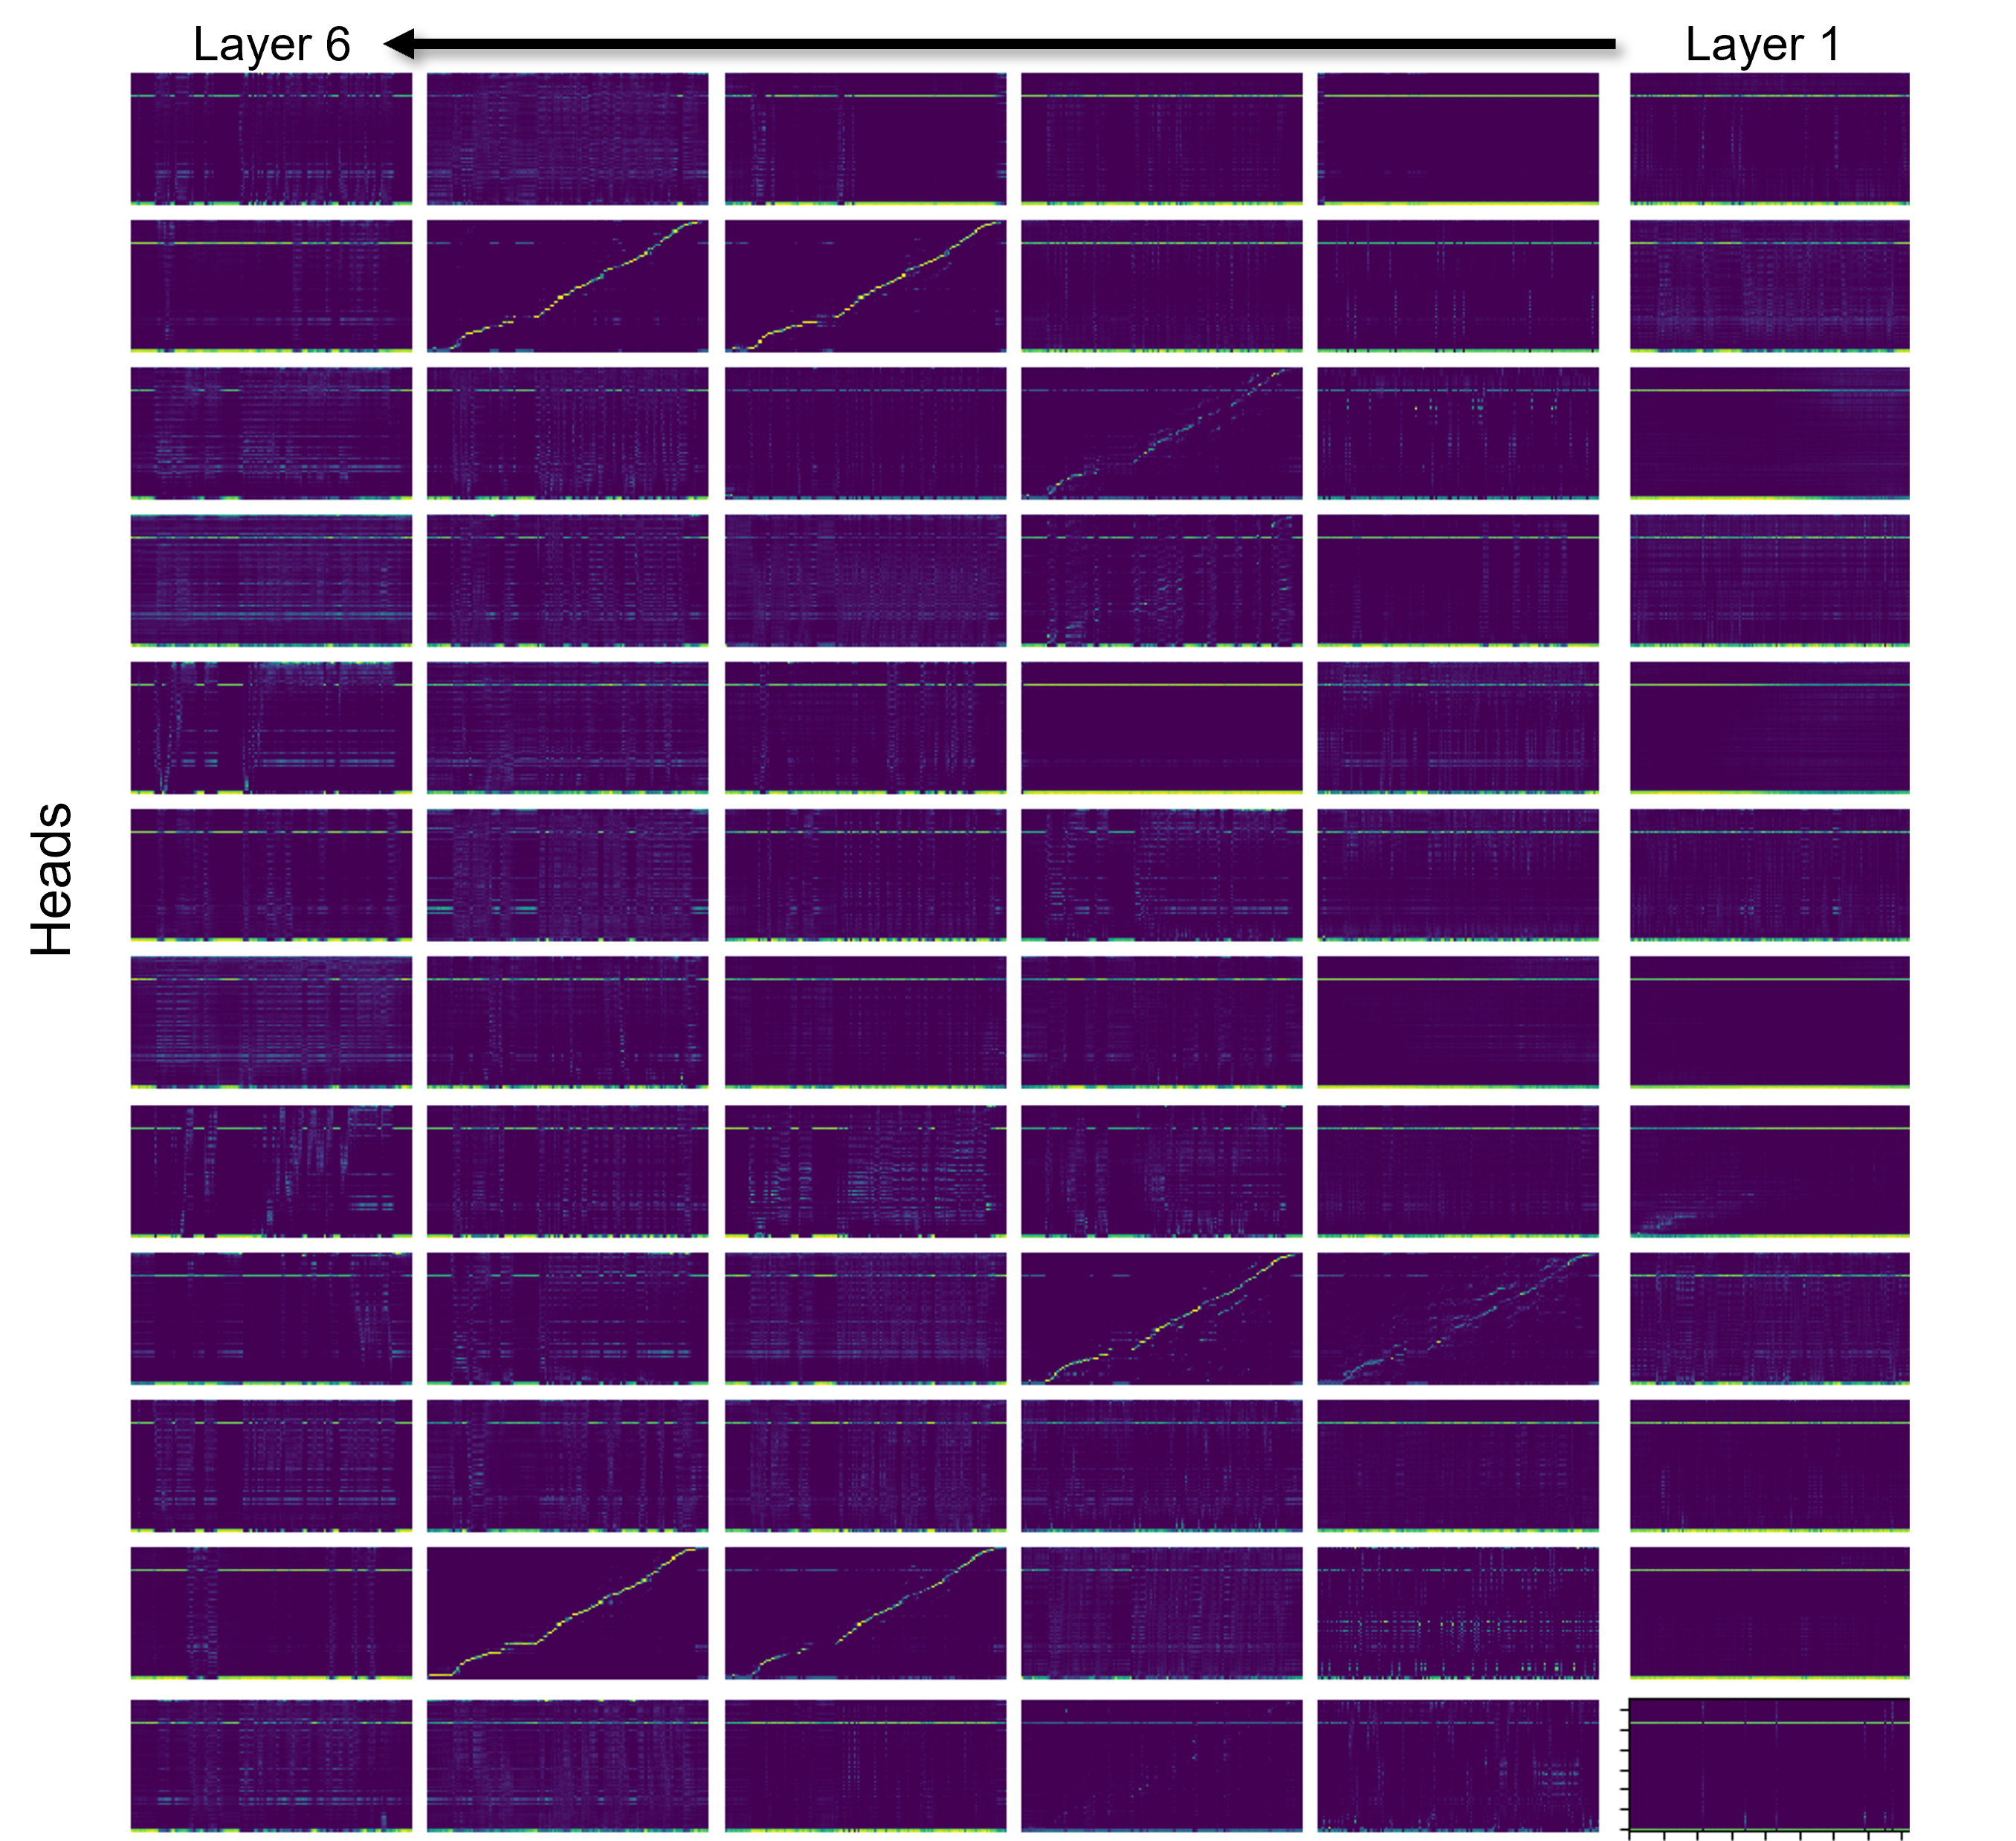}
    \caption{Training cross-attention alignment of all heads and all layers of Transformer TTS.}
    \label{fig:appen:transformertts}
\end{figure*}
