# Supplementary material for: A Vector Quantized Approach for Text to Speech Synthesis on Real-World Spontaneous Speech
Source: arXiv:2302.04215 source file (2023-02-08)
Supplement: Supplementary file 2 [file appendix-vqtts-alignment.tex]

\begin{figure*}[!tb]
    \centering
    \includegraphics[width=\textwidth]{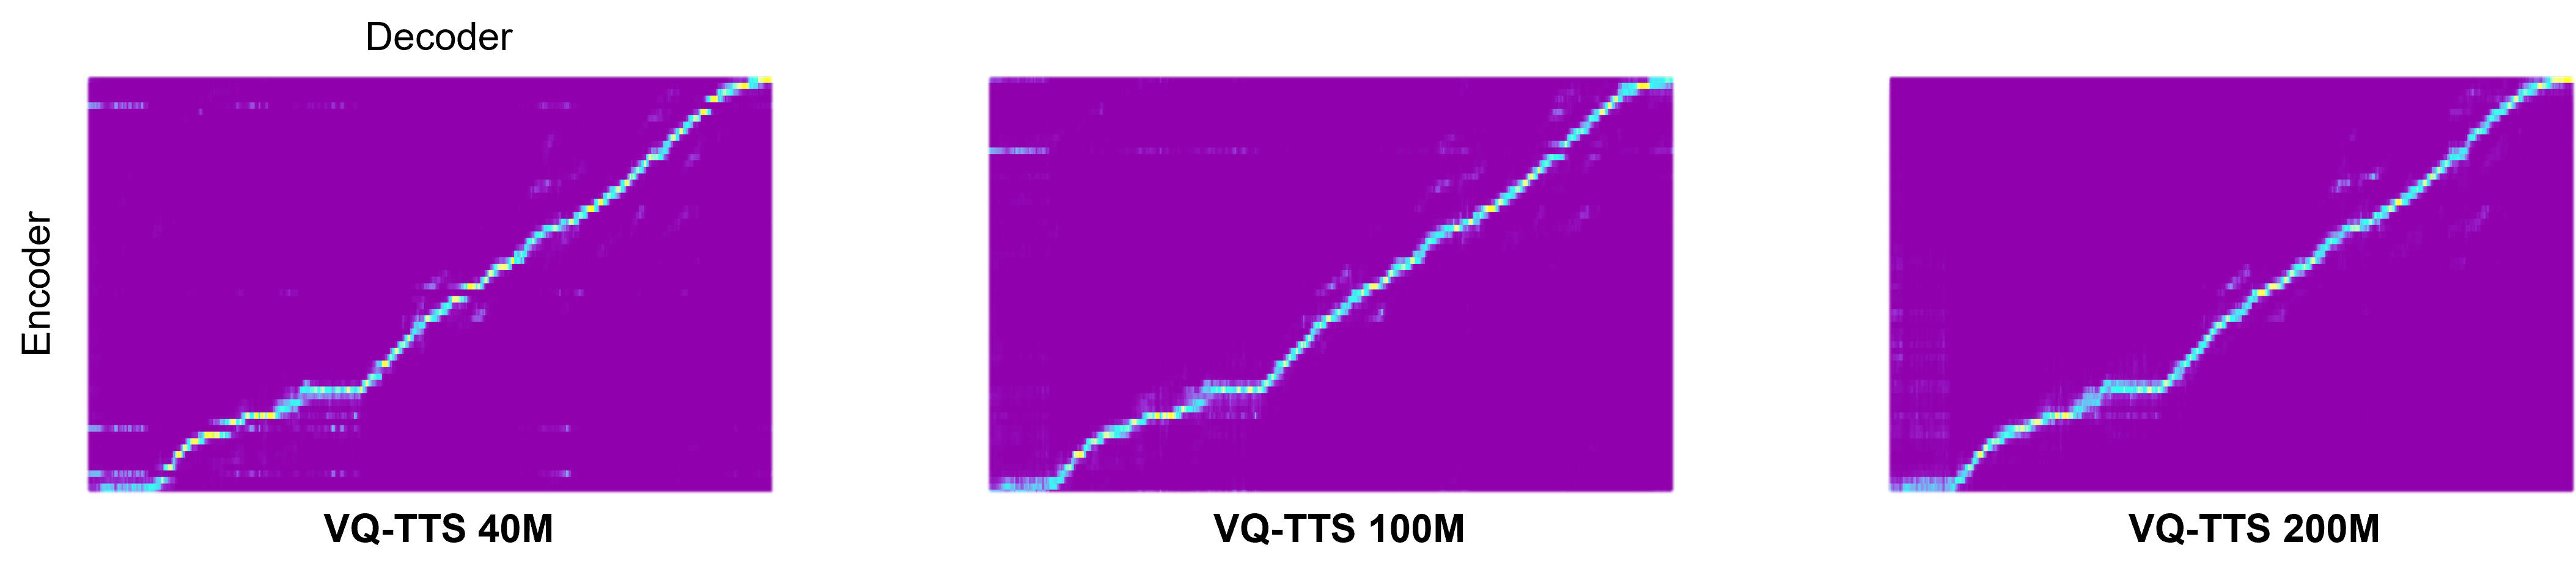}
    \caption{Comparison of training encoder-decoder alignment of VQ-TTS of different parameter size in the same utterance. We increase the brightness and contrast for better visualization on the difference.}
    \label{fig:appen:vqtts-alignment}
\end{figure*}
